# Supplementary material for: BioNetGen 2.2: Advances in Rule-Based Modeling
Source: arXiv:1507.03572 ancillary file (2016-07-01)
Supplement: Supplementary file 1 [file Supplementary_text.pdf]

# SUPPLEMENTARY INFORMATION

## BioNetGen 2.2: Advances in Rule-Based Modeling

Leonard A. Harris, Justin S. Hogg, José-Juan Tapia, John A. P. Sekar, Sanjana A. Gupta, Ilya Korsunsky, Arshi Arora, Dipak Barua, Robert P. Sheehan, and James R. Faeder*

Department of Computational and Systems Biology, University of Pittsburgh School of Medicine, Pittsburgh, PA, USA

*Corresponding author: faeder@pitt.edu

## General Information

BioNetGen website: bionetgen.org

Source code: github.com/RuleWorld/bionetgen

Release notes: bionetgen.org/index.php/Release_Notes

Users' email list: groups.google.com/d/forum/bionetgen-users

Developers' email list: groups.google.com/d/forum/RuleWorld-developers

Facebook: facebook.com/bionetgen

Twitter: twitter.com/bionetgen

## Online Documentation

Actions & Arguments Guide: bionetgen.org/index.php/BNG_Actions_Args

Built-in mathematical operators and functions: bionetgen.org/index.php/Built-ins

Compartmental BNGL: bionetgen.org/index.php/Compartments_in_BNGL

Energy-based modeling: bionetgen.org/index.php/Energy_Modeling

Functional rate laws: bionetgen.org/index.php/Functions

Hybrid particle/population (HPP): bionetgen.org/index.php/HPP

MEX code generation: bionetgen.org/index.php/Mex_code_generator

Partial list of publications using BioNetGen: /bionetgen.org/index.php/Model_Examples

Partitioned leaping: bionetgen.org/index.php/RK-PLA

SBML-to-BNGL translation (Atomizer): bionetgen.org/index.php/SBML2BNGL

Spatial modeling with CellBlender/MCell: bionetgen.org/index.php/Compartmental_LR_model

Visualization: bionetgen.org/index.php/Visualization

# Runge-Kutta PLA

The partitioned-leaping algorithm (PLA) [1] is a multiscale variant of the $\tau$-leaping algorithm of Gillespie [2, 3]. The PLA differs from other $\tau$-leaping variants (e.g., [4–11]) in that it utilizes the full theoretical framework derived by Gillespie [12] for bridging from the exact-stochastic to the continuous-deterministic description of chemical kinetics. At each step of a PLA simulation, each reaction is classified, based on the current values of the reaction rate and the time step, into one of four categories spanning both discrete and continuous representations: *exact stochastic*, *Poisson*, *Langevin*, and *deterministic*. As such, the PLA is able to efficiently "leap" over large numbers of reaction firings involving species with large populations (e.g., metabolites, small-molecule signaling agents) while simultaneously accurately capturing stochastic effects associated with small-population species (e.g., genes, mRNA transcripts). An extensive performance analysis comparing the PLA to the exact stochastic simulation algorithm (SSA) [13] is presented in [14]. A spatial variant of the PLA has also been proposed [15]. Further information regarding the theoretical foundations of the PLA can be found in [16].

In its original formulation, the $\tau$-leaping algorithm (and many of its variants, including the PLA) is analogous to the simple forward Euler method for solving ordinary differential equations (ODEs) [2]. Recognizing the potential limitations that this poses, Gillespie proposed in [2] an additional method, termed the "midpoint" $\tau$-leaping algorithm, based on estimating the values of the reaction propensities (rates) at the midpoint between time $t$ (the current time) and $t + \tau$, where $\tau$ is the chosen time step. This method is analogous to the well known midpoint method for solving ODEs, which is a second-order variant of a larger class of methods known as explicit Runge-Kutta methods [17]. This generalization of the original $\tau$-leaping algorithm has inspired the development of numerous additional $\tau$-leaping methods, including implicit [18, 19] and higher-order Runge-Kutta [20] variants. An in-depth discussion of different $\tau$-leaping variants and their relationship to the PLA can be found in [16].

In BioNetGen 2.2, we have followed this lead and implemented an explicit Runge-Kutta variant of the PLA (RK-PLA). Details of the implementation will be reported elsewhere [21]. However, briefly, the algorithm is comprised of four basic steps:

1. $\tau$ selection (time step calculation)
2. reaction classification
3. firing generation
4. postleap checking and correcting

$\tau$ selection can be performed using either established pre-leap $\tau$-selection formulae [1, 4] or via a postleap checking strategy similar to that proposed by Anderson [22]. Both approaches require defining various adjustable parameters (see Table S1), including the "error control parameter" $\epsilon$ [2], and can be invoked in either a reaction-based (RB) or species-based (SB) formulation [1, 4]. Reaction classification and firing generation depend on the calculated values of $\tau$ and the chosen Runge-Kutta method. Forward Euler (first order), midpoint (second order), and 4th-order Runge-Kutta methods can be called by keyword (Table S1). Custom methods (explicit only) can also be defined in a Butcher tableau [17] input file. Postleap checking can be performed in two ways: (i) a simple check to ensure that populations do not become negative [23]; (ii) a check to see if the so-called "leap condition" [2] (either RB or SB versions [1, 4]) has been violated. Negative-population postleap checking can only be performed in concert with pre-leap $\tau$ selection. Leap-condition, or "$\epsilon$-based," postleap checking can be performed either with pre-leap $\tau$ selection or within a full Anderson-style postleap checking procedure [22]. In all cases, postleap violations are corrected using binomial random numbers, as in [22].

BioNetGen 2.2 users can perform RK-PLA simulations by calling either the `simulate_pla` action or the `simulate` action together with the `method=>"pla"` argument (Table S2), invoked in the usual way from within a `.bngl` input file [24]. In both cases, a user-defined configuration of $\tau$-selection, reaction classification, firing generation, and postleap checking/correcting methods can be defined through the `pla_config` argument (Table S2), which takes a string subdivided into three parts separated by vertical bars,

```
pla_config=>"arg1|arg2|arg3",
```

where `arg1` specifies the desired Runge-Kutta method, `arg2` defines a $\tau$ selection + postleap checking/correcting combination, and `arg3` is reserved for parameter definitions. If not defined, the default configuration is

pla_config=>"fEuler|pre-neg:sb|eps=0.03", which specifies a forward Euler method with SB pre-leap $\tau$ selection, negative-population postleap checking, and an error control parameter $\epsilon = 0.03$. A complete list of pla_config arguments is provided in Table S1.

As a first test of the RK-PLA implementation in BioNetGen 2.2, we performed a weak-order error analysis using the simple test system $S \xrightarrow{k=1} 2S$, with initial population $X(0) = 1$. We ran 100 000 RK-PLA simulations to $t = 8$ using four RK methods, ranging from first to fourth order, with a negative-population postleap checker and a range of fixed time steps between 0.01 and 8. The first-, second-, and fourth-order methods are the forward Euler, midpoint, and 4th-order Runge-Kutta methods supported by keyword. We also considered Kutta's 3rd-order method [17], specified via a Butcher tableau input file. We performed an equal number of SSA simulations and calculated the RK-PLA error in the first moment ($|E[X_{PLA}(8)] - E[X_{SSA}(8)]|$) and second moment ($\left|E[X^2_{PLA}(8)] - E[X^2_{SSA}(8)]\right|$) as a function of the time step. In Fig. S1a, we see that the error in the first moment scales as expected for each method (slope $\leq$ order). In Fig. S1b, the error in the second moment scales as first order in all cases.

We then tested the RK-PLA simulator on the decaying-dimerizing (DD) reaction set [2], a model comprised of the following four reactions,

$$\begin{aligned} S_1 &\xrightarrow{k_1} 0, \\ S_1 + S_1 &\underset{k_3}{\overset{k_2}{\rightleftharpoons}} S_2, \\ S_2 &\xrightarrow{k_4} S_3, \end{aligned}$$

where $k_1 = 1.0\ \mathrm{s}^{-1}$, $k_2 = 0.002\ \mathrm{s}^{-1}$, $k_3 = 0.5\ \mathrm{s}^{-1}$, and $k_4 = 0.04\ \mathrm{s}^{-1}$. The initial species populations are $X_1(0) = 4150$, $X_2(0) = 39\,565$, and $X_3(0) = 3445$ [2]. Simulations were run to $t = 30$ s using the forward Euler variant of the RK-PLA with SB pre-leap $\tau$ selection, negative-population postleap checking, and values of the error-control parameter $\epsilon = [\,0.01,\ 0.03,\ 0.05,\ 0.1,\ 0.2\,]$. For each value of $\epsilon$, we ran 10 000 RK-PLA simulations and generated smoothed histograms [1] for $X_1(10)$, the population of species $S_1$ at $t = 10$ s. We also generated histograms from 10 000 SSA simulations for comparison. Differences between the RK-PLA and SSA histograms were quantified using the "histogram distance," $D$, and the "self distance," $D_{\mathrm{self}}$ [1, 25]. Two histograms cannot be statistically distinguished if $D \leq D_{\mathrm{self}}$. In Fig. S2a, we show the mean time course for species $S_1$ from 10 000 SSA simulations. In Fig. S2b, we plot the ratio of the RK-PLA and SSA run times for each value of $\epsilon$. We also include next to each symbol values of the histogram distance $D$. Circles are used if $D \leq D_{\mathrm{self}}$ and triangles are used otherwise. We see in Fig. S2b that for $\epsilon = 0.05$ we achieve a speedup of $\sim 4\times$ with no loss of accuracy; for $\epsilon = 0.1$ we achieve a speedup of $\sim 8\times$ with minimal loss of accuracy. Increasing the order of the RK method does not significantly improve accuracy in this case.

As a final test of the RK-PLA simulator, we considered a published model of epidermal growth factor (EGF) receptor (EGFR)-mediated signaling [26, 27] (available in the Models2 directory of the BioNetGen 2.2.6 release as egfr_path.bngl). The primary focus of this model is the cascade of signaling events that leads to recruitment of cytosolic Sos to the inner cell membrane. EGF ligands bind to EGFR, leading to the formation of signaling-competent receptor dimers, which can be transphoshorylated. The cytosolic adapter proteins Grb2 and Shc are recruited to the phosphorylated dimer. When Shc is bound to a dimer it can be phosphorylated by EGFR. The phosphorylated form of Shc interacts with Grb2, which interacts constitutively with Sos. The model is comprised of 18 species (EGF, EGFR, Grb2, Shc, Sos + complexes) and 37 reactions. We performed RK-PLA simulations using SB pre-leap $\tau$ selection, negative-population postleap checking, and values of the error-control parameter $\epsilon = [\,0.01,\ 0.03,\ 0.05,\ 0.1,\ 0.2\,]$. To illustrate the advantages of using a higher-order RK method, we performed simulations using both the forward Euler and midpoint variants of the RK-PLA. For each configuration, we ran 10 000 RK-PLA and SSA simulations to $t = 100$ s and compared histograms for activated Sos (Sos_act) at $t = 10$ s using the histogram and self distances. In Fig. S3a, we show the mean time course for activated Sos from 10 000 SSA simulations. In Fig. S3b, we show that for forward Euler with $\epsilon = 0.05$ we achieve a speedup of $\sim 8\times$ with respect to the SSA with no loss of accuracy. In Fig. S3c, we show that with the higher-order midpoint method we can increase $\epsilon$ to 0.1 with no loss of accuracy, resulting in a speedup of $> 20\times$. Further increasing the order of the method has no significant effect on the accuracy in this case.

The examples that we have presented here demonstrate the ability of the RK-PLA simulator in BioNetGen 2.2 to perform accurate and efficient stochastic simulations on select models. A more extensive performance

analysis considering additional RK-PLA features (`pre-eps`/`post-eps` configurations, higher-order methods, etc.), as well as more complex models, will be presented elsewhere [21]. However, some practical rules-of-thumb that we can report here based on our experiences include: (i) values of $\epsilon$ between 0.03 and 0.1 provide a good balance between accuracy and efficiency in most cases; (ii) all else being equal, simulation run times increase (as expected) with increasing order of the RK method (`fEuler` < `midpoint` < `kutta3` < `rk4`); (iii) SB methods tend to be somewhat faster than equivalent RB methods; (iv) `pre-eps` configurations tend to be the slowest but most accurate, `post-eps` methods tend to be the fastest but least accurate, and `pre-neg` methods lie somewhere in between. Further documentation about the RK-PLA simulator in BioNetGen 2.2 can be found at bionetgen.org/index.php/RK-PLA. User questions can be directed to bionetgen.help@gmail.com.

# References


[1] L. A. Harris and P. Clancy, "A 'partitioned leaping' approach for multiscale modeling of chemical reaction dynamics," *J. Chem. Phys.*, vol. 125, p. 144107, 2006.

[2] D. T. Gillespie, "Approximate accelerated stochastic simulation of chemically reacting systems," *J. Chem. Phys.*, vol. 115, pp. 1716–1733, 2001.

[3] D. T. Gillespie, "Stochastic simulation of chemical kinetics," *Annu. Rev. Phys. Chem.*, vol. 58, pp. 35–55, 2007.

[4] Y. Cao, D. T. Gillespie, and L. R. Petzold, "Efficient step size selection for the tau-leaping simulation method," *J. Chem. Phys.*, vol. 124, p. 044109, 2006.

[5] T. Tian and K. Burrage, "Binomial leap methods for simulating stochastic chemical kinetics," *J. Chem. Phys.*, vol. 121, pp. 10356âĂŞ–10364, 2004.

[6] A. Chatterjee, D. G. Vlachos, and M. A. Katsoulakis, "Binomial distribution based $\tau$-leap accelerated stochastic simulation," *J. Chem. Phys.*, vol. 122, p. 024112, 2005.

[7] A. Auger, P. Chatelain, and P. Koumoutsakos, "R-leaping: Accelerating the stochastic simulation algorithm by reaction leaps," *J. Chem. Phys.*, vol. 125, p. 084103, 2006.

[8] X. Cai and Z. Xu, "K-leap method for accelerating stochastic simulation of coupled chemical reactions," *J. Chem. Phys.*, vol. 126, p. 074102, 2007.

[9] M. F. Pettigrew and H. Resat, "Multinomial tau-leaping method for stochastic kinetic simulations," *J. Chem. Phys.*, vol. 126, p. 084101, 2007.

[10] X. Peng, W. Zhou, and Y. Wang, "Efficient binomial leap method for simulating chemical kinetics," *J. Chem. Phys.*, vol. 126, p. 224109, 2007.

[11] A. Leier, T. T. Marquez-Lago, and K. Burrage, "Generalized binomial $\tau$-leap method for biochemical kinetics incorporating both delay and intrinsic noise," *J. Chem. Phys.*, vol. 128, p. 205107, 2008.

[12] D. T. Gillespie, "The chemical Langevin equation," *J. Chem. Phys.*, vol. 113, pp. 297–306, 2000.

[13] D. T. Gillespie, "A general method for numerically simulating the stochastic time evolution of coupled chemical reactions," *J. Comput. Phys.*, vol. 22, pp. 403–434, 1976.

[14] L. A. Harris, A. M. Piccirilli, E. R. Majusiak, and P. Clancy, "Quantifying stochastic effects in biochemical reaction networks using partitioned leaping," *Phys. Rev. E*, vol. 79, p. 051906, 2009.

[15] K. A. Iyengar, L. A. Harris, and P. Clancy, "Accurate implementation of leaping in space: the spatial partitioned-leaping algorithm," *J. Chem. Phys.*, vol. 132, p. 094101, 2010.

[16] L. A. Harris, *Multiscale Simulation of Reaction Dynamics in Chemical, Biological and Materials Systems.* PhD thesis, Cornell University, 2010.

[17] J. C. Butcher, *Numerical Methods for Ordinary Differential Equations.* Chichester, UK.: John Wiley & Sons, Ltd, 2nd ed., 2008.

[18] M. Rathinam, L. R. Petzold, Y. Cao, and D. T. Gillespie, "Stiffness in stochastic chemically reacting systems: The implicit tau-leaping method," *J. Chem. Phys.*, vol. 119, pp. 12784–12794, 2003.

[19] Y. Cao, L. R. Petzold, M. Rathinam, and D. T. Gillespie, "The numerical stability of leaping methods for stochastic simulation of chemically reacting systems," *J. Chem. Phys.*, vol. 121, pp. 12169–12178, 2004.

[20] K. Burrage and T. Tian, "Poisson Runge-Kutta methods for chemical reaction systems," in *Third International Workshop on Scientific Computing and Applications* (Y. Lu, W. Sun, and T. Tang, eds.), vol. 1 of *Advances in Scientific Computing and Applications*, pp. 82–96, Science Press, 2004.

[21] L. A. Harris, S. Gupta, L. J. Stover, N. S. Nair, and J. R. Faeder, "An explicit Runge-Kutta $\tau$-leaping algorithm." *in preparation.*

[22] D. F. Anderson, "Incorporating postleap checks in tau-leaping," *J. Chem. Phys.*, vol. 128, p. 054103, 2008.

[23] Y. Cao, D. T. Gillespie, and L. R. Petzold, "Avoiding negative populations in explicit Poisson tau-leaping," *J. Chem. Phys.*, vol. 123, p. 054104, 2005.

[24] J. R. Faeder, M. L. Blinov, and W. S. Hlavacek, "Rule-based modeling of biochemical systems with BioNetGen," in *Methods in Molecular Biology*, vol. 500, pp. 113–167, Clifton, N.J.: Humana Press, 2009.

[25] Y. Cao and L. Petzold, "Accuracy limitations and the measurement of errors in the stochastic simulation of chemically reacting systems," *J. Comput. Phys.*, vol. 212, pp. 6–24, 2006.

[26] B. N. Kholodenko, O. V. Demin, G. Moehren, and J. B. Hoek, "Quantification of short term signaling by the epidermal growth factor receptor," *J. Biol. Chem.*, vol. 274, pp. 30169–30181, 1999.

[27] M. L. Blinov, J. R. Faeder, B. Goldstein, and W. S. Hlavacek, "A network model of early events in epidermal growth factor receptor signaling that accounts for combinatorial complexity," *Biosystems*, vol. 83, pp. 136–151, 2006.

Table S1: List of all supported options to the `pla_config` argument in BioNetGen 2.2. If `pla_config` is not defined in the `simulate_pla` or `simulate` action call then a default configuration of `"fEuler|pre-neg:sb|eps=0.03"` is used. All keywords are *case-insensitive*.

## `pla_config=>"arg1|arg2|arg3"`

| **`arg1`** | |
|---|---|
| `fEuler` | forward Euler |
| `midpt` | midpoint |
| `rk4` | 4th-order Runge-Kutta |
| `custom` | custom method (requires `bt` to be defined) |

| **`arg2`** | |
|---|---|
| `pre-neg:rb` | RB pre-leap $\tau$ selection + negative-population postleap checking |
| `pre-neg:sb` | SB pre-leap $\tau$ selection + negative-population postleap checking |
| `pre-eps:rb` | RB pre-leap $\tau$ selection + $\epsilon$-based (leap condition) postleap checking |
| `pre-eps:sb` | SB pre-leap $\tau$ selection + $\epsilon$-based (leap condition) postleap checking |
| `post-eps:rb` | RB Anderson-style postleap checking/$\tau$ selection |
| `post-eps:sb` | SB Anderson-style postleap checking/$\tau$ selection |
| `Anderson:rb` | same as `post-eps:rb` |
| `Anderson:sb` | same as `post-eps:sb` |
| `fixed-neg` | fixed time step + negative-population postleap checking (requires `tau` to be defined) |
| `fixed-eps:rb` | fixed time step + RB $\epsilon$-based postleap checking (requires `tau` to be defined) |
| `fixed-eps:sb` | fixed time step + SB $\epsilon$-based postleap checking (requires `tau` to be defined) |

| **`arg3`** (comma-separated list: `par1=val1,par2=val2,...`) | |
|---|---|
| `eps` | "error-control parameter" ($0 \lesssim \epsilon < 1$); used in pre-leap $\tau$ selection and $\epsilon$-based postleap checking; *required* |
| `apx1` | "approximately 1" ($\approx$1); used in reaction classification; *default*: 3 |
| `gg1` | "much greater than 1" ($\gg$1); used in reaction classification; *default*: 100 |
| `p` | fraction to reduce $\tau$ if postleap violation is detected; *default*: 0.5 |
| `pp` | fraction to reduce $\tau$ if postleap leap check is "barely" satisfied (`post-eps:rb`, `post-eps:sb` only); *default*: 0.8 |
| `q` | fraction to increase $\tau$ if postleap leap check is "substantially" satisfied (`post-eps:rb`, `post-eps:sb` only); *default*: 1.5 |
| `w` | fraction of leap condition that if satisfied is considered "substantial" (`post-eps:rb`, `post-eps:sb` only); *default*: 0.75 |
| `tau` | fixed time step (required for `fixed-neg`, `fixed-eps:rb`, `fixed-eps:sb`) |
| `bt` | Butcher tableau input file (including path; required for `custom`) |

Figure S1: Weak-order error analysis of the RK-PLA implementation in BioNetGen 2.2 using the simple test system $S \xrightarrow{k=1} 2S$, with initial population $X(0)=1$: (a,b) errors in the first (a) and second (b) moments as a function of the time step; (c) Butcher tableau for Kutta's 3rd-order method [17]; (d) Butcher tableau input file used to run RK-PLA simulations with Kutta's 3rd-order method. In (a,b), all plotted points are based on 100 000 RK-PLA and SSA simulations run to $t = 8$. RK-PLA simulations were performed with fixed time steps and a negative-population postleap checker, i.e., `pla_config=>"METHOD|fixed-neg|tau=FLOAT"` for `METHOD` = `fEuler`, `midpt`, `rk4` and `pla_config=>"custom|fixed-neg|tau=FLOAT,bt=[path_to_file]/ButcherTableau.txt"` for Kutta's 3rd-order method. In all cases, $0.01 \leq$ `FLOAT` $\leq 8$. (`fEuler`: forward Euler; `midpt`: midpoint; `kutta3`: Kutta's 3rd-order; `rk4`: 4th-order Runge-Kutta.)

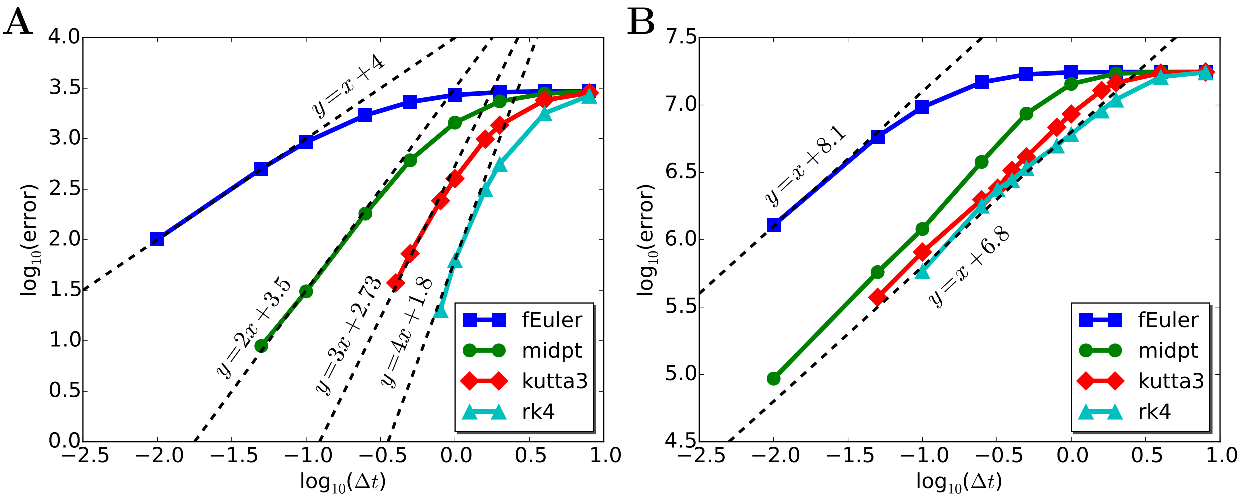


**C**

kutta3

| | | | |
|---|---|---|---|
| 0 | | | |
| ½ | ½ | | |
| 1 | -1 | 2 | |
| | ⅙ | ⅔ | ⅙ |

**D**

ButcherTableau.txt

```
0    0    0
1/2  0    0
-1   2    0
#-----------
1/6  2/3  1/6
```

Figure S2: Performance analysis for the decaying-dimerizing (DD) reaction set: (a) average time course for species $S_1$ from 10 000 SSA simulations; (b) ratio of RK-PLA to SSA run times as a function of error-control parameter $\epsilon$. In (b), values of the histogram distance $D$ are shown next to the symbols for each value of $\epsilon$; circles are used if $D \leq D_{\mathrm{self}}$, triangles are used otherwise. Smoothed histograms at $t = 10$ s are shown in the inset, with colors corresponding to those of the symbols in the main plot. Mean values are designated with '+'; horizontal bars represent $\pm$ one standard deviation around the mean. The SSA histogram is shown in black. All histograms were generated using the histogram smoothing procedure described in [1] with a "smoothing parameter" $\sigma = 30$. RK-PLA simulations were run with `pla_config=>"fEuler|pre-neg:sb|eps=FLOAT"`, where `FLOAT` is one of `[0.01,0.03,0.05,0.1,0.2]`.

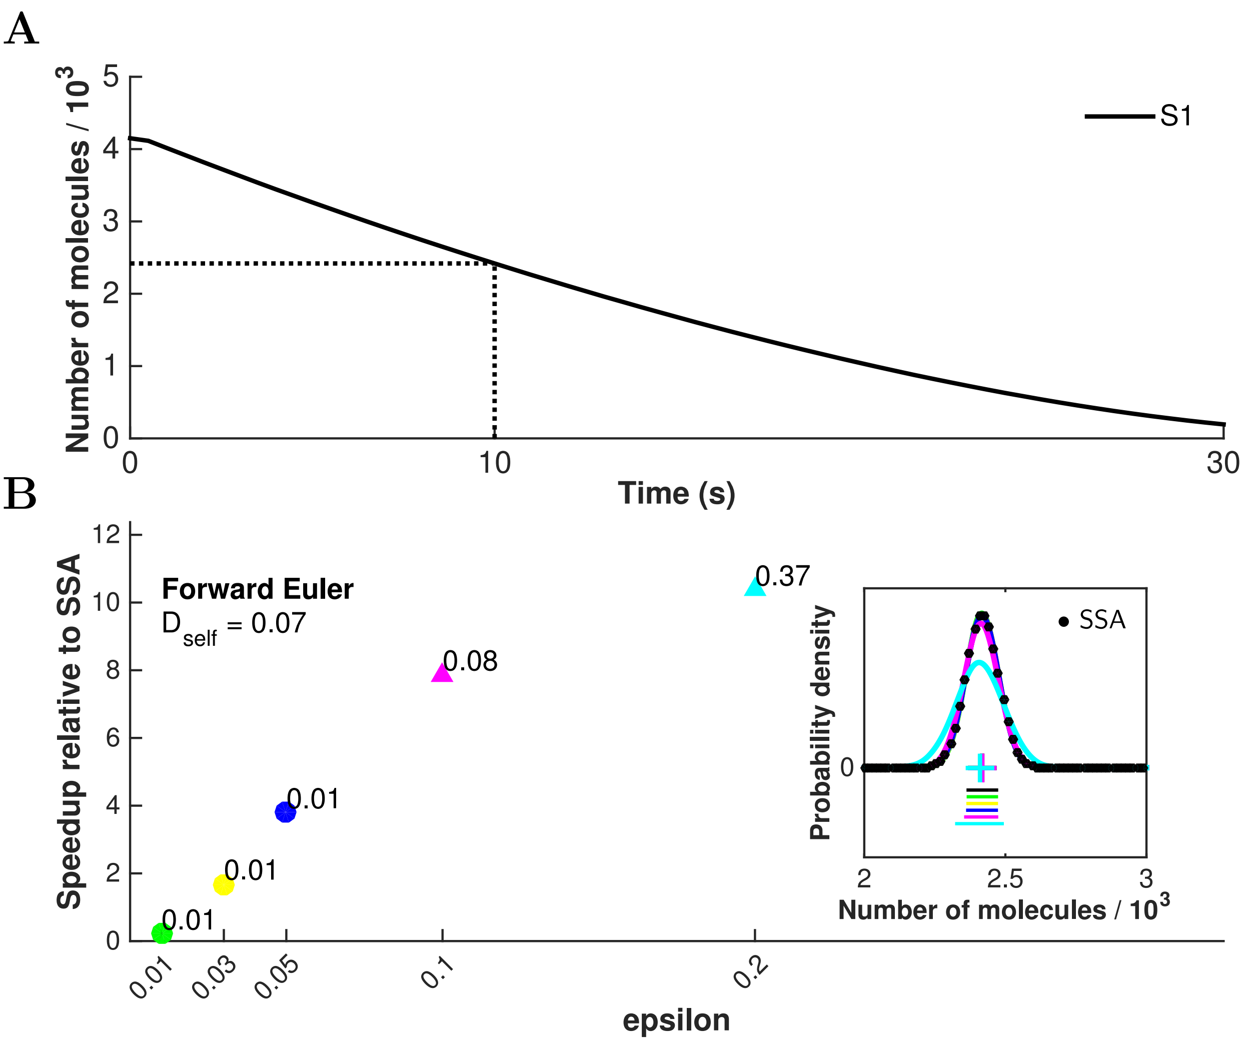

Figure S3: Performance analysis for the EGFR signaling model [26, 27]: (a) average time course for activated Sos from 10 000 SSA simulations; (b,c) ratio of RK-PLA to SSA run times as a function of error-control parameter $\epsilon$ for the forward Euler and midpont RK-PLA variants. Layout is identical to that in Fig. S2. All smoothed histograms were generated with a "smoothing parameter" $\sigma = 30$. RK-PLA simulations were run with `pla_config=>"METHOD|pre-neg:sb|eps=FLOAT"`, where `METHOD` is `fEuler` or `midpt` and `FLOAT` is one of `[0.01,0.03,0.05,0.1,0.2]`.

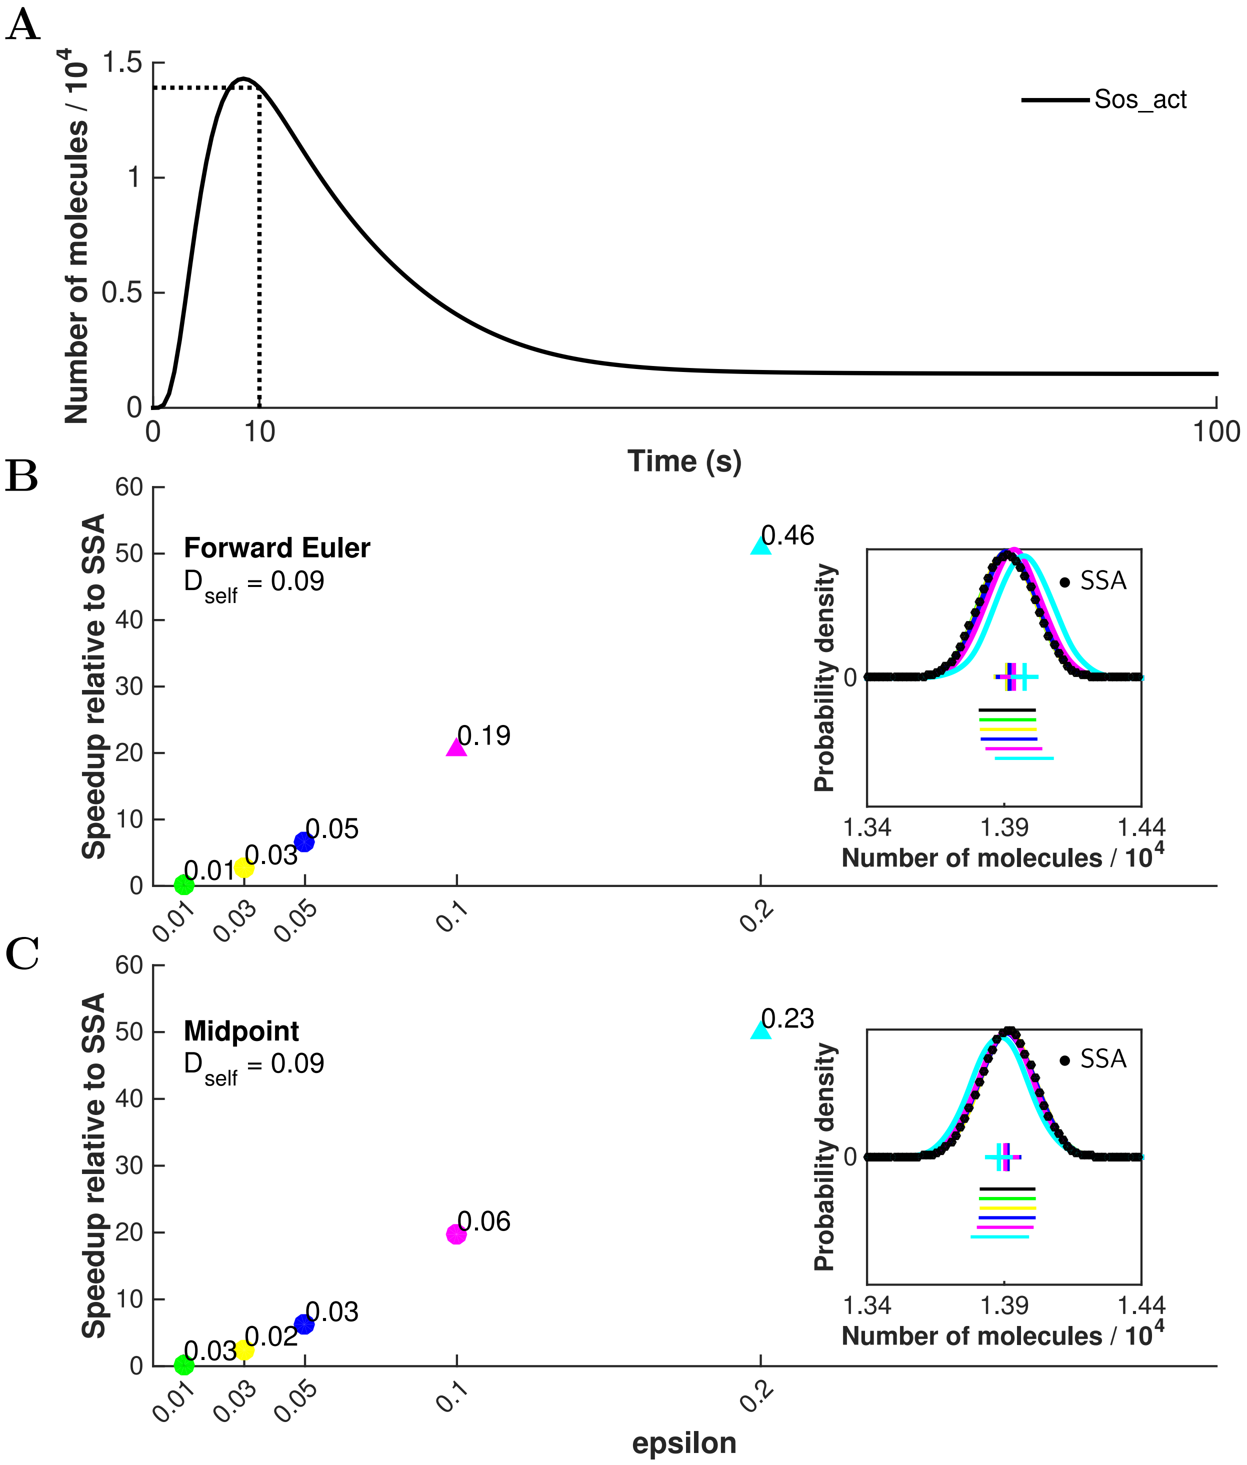

Table S2: New actions and arguments (`key=>value` format) introduced in the BioNetGen 2.2.x series of releases. `STRING` is any string of characters (must be enclosed in quotes); `INT` is any integer; `FLOAT` is any real-valued number; `BOOL` is either 0 (False) or 1 (True); `[...]` is a comma-separated list. Default values are provided for optional arguments. Actions introduced prior to version 2.2.0 are labeled "`< 2.2.0`". For a complete list of all BioNetGen actions and arguments, see [http://bionetgen.org/index.php/BNG_Actions_Args](http://bionetgen.org/index.php/BNG_Actions_Args).

| `action({argument=>type})` | **Description** | **Introduced** |
|---|---|---|
| `bifurcate({})` | Perform a bifurcation analysis.<br>*Inherits all arguments from* `parameter_scan`, *with the following defaults*:<br>`reset_conc=>0` | `2.2.6` |
| `generate_hybrid_model({` | Generate a hybrid particle/population version of a BNGL model.<br>*Significantly reduces memory use in NFsim simulations.* | `2.2.0` |
| `prefix=>"STRING",` | Change the base filename for output.<br>**Default**: *model name* | `2.2.0` |
| `suffix=>"STRING",` | Suffix added to output base filename.<br>**Default**: `"hpp"` | `2.2.0` |
| `actions=>["STRING",...],` | List of actions to append to bottom of generated hybrid model file.<br>**Default**: `"writeXML()"` | `2.2.0` |
| `execute=>BOOL,` | Execute actions in hybrid model.<br>**Default**: `0` | `2.2.0` |
| `overwrite=>BOOL,` | Overwrite existing hybrid model file.<br>**Default**: `0` | `2.2.0` |
| `safe=>BOOL,` | Enable safe mode.<br>*Less efficient but guaranteed to work with any "lumping rate constant" value.*<br>**Default**: `0` | `2.2.4` |
| `verbose=>BOOL`<br>`})` | Enable verbose output.<br>**Default**: `0` | `2.2.0` |
| `parameter_scan({` | Scan over a range of values of a specified parameter.<br>*Recognizes all previous arguments (including all from* `simulate`*), plus ...* | `< 2.2.0` |
| `par_scan_vals=>[FLOAT,...],` | Specific values of a parameter to be scanned over.<br>(*Required if* `par_min`, `par_max`, and `n_scan_pts` *not defined.*)<br>**Default**: *N/A* | `2.2.6` |
| `reset_conc=>BOOL`<br>`})` | Reset species concentrations after each simulation of a scan.<br>**Default**: `1` | `2.2.6` |
| `readFile({` | Read a model from file.<br>*Recognizes all previous arguments, plus ...* | `< 2.2.0` |
| `blocks=>["STRING",...],` | List of blocks to be read in from a BNGL or NET file.<br>**Default**: *all blocks* | `2.2.6` |
| `atomize=>BOOL`<br>`})` | Import an SBML model as "flat" (`atomize=>0`) or structured (`atomize=>1`).<br>**Default**: `0` | `2.2.6` |
| `simulate_pla({` | Simulate using the "partitioned-leaping algorithm" (PLA), a $\tau$-leaping variant.<br>*Inherits many arguments from* `simulate_ode` *and* `simulate_ssa`, *plus ...* | `2.2.0` |
| `pla_config=>"STRING"`<br>`})` | Define configuration parameters needed to run PLA simulations.<br>**Default**: `"fEuler\|pre-neg:sb\|eps=0.03"` | `2.2.0` |
| `simulate({` | All-purpose simulate action.<br>*Inherits all arguments from* `simulate_ode`, `simulate_ssa`, `simulate_pla`, *and* `simulate_nf`, *plus ...* | `2.2.0` |
| `method=>"STRING",` | Set simulation method as `"ode"`, `"ssa"`, `"pla"`, or `"nf"`.<br>*Required argument.* | `2.2.0`<br>(`"nf"` *in* `2.2.6`) |
| `argfile=>"STRING",` | File name containing action commands and arguments.<br>**Default**: *N/A* | `2.2.0` |
| `max_sim_steps=>INT,` | Maximum number of simulation steps.<br>**Default**: *N/A* | `2.2.0` |

| | | |
|---|---|---|
| `output_step_interval=>INT,` | Number of simulation steps between outputs.<br>**Default**: *N/A* | 2.2.0 |
| `print_CDAT=>BOOL,` | Print species concentrations to `.cdat` file at all output times.<br>(*If* `print_CDAT=>0`, *only initial and final concentrations are printed.*)<br>**Default**: `1` | 2.2.0 |
| `print_functions=>BOOL,` | Print values of global functions to `.gdat` file at all output times.<br>**Default**: `0` | 2.2.0 |
| `print_on_stop=>BOOL,` | Print to file at the time point that logical stopping condition is met.<br>**Default**: `1` | 2.2.1 |
| `stop_if=>"STRING"`<br>`})` | Define a logical condition for terminating a simulation.<br>**Default**: *N/A* | 2.2.1 |
| `writeFile({` | All-purpose method for writing models to file. | 2.2.0 |
| `format=>"STRING",` | Select output format as `"bngl"`, `"net"`, or `"xml"`.<br>(`"xml"` *writes BNG-XML, readable by NFsim; for SBML, use* `writeSBML`.)<br>**Default**: `"net"` | 2.2.0 |
| `prefix=>"STRING",` | Set prefix of output file name.<br>**Default**: *model name* | 2.2.0 |
| `suffix=>"STRING",` | Set suffix of output file name.<br>**Default**: *N/A* | 2.2.0 |
| `include_model=>BOOL,` | Include model blocks in output file.<br>**Default**: `1` | 2.2.0 |
| `include_network=>BOOL,` | Include network blocks in output file.<br>**Default**: `1` | 2.2.0 |
| `evaluate_expressions=>BOOL,` | Evaluate mathematical expressions to numbers.<br>**Default**: `0` | 2.2.0 |
| `pretty_formatting=>BOOL,` | Write output in human-readable form.<br>**Default**: `1` | 2.2.0 |
| `TextReaction=>BOOL,` | Write reactions as BNGL strings.<br>**Default**: `0` | 2.2.0 |
| `TextSpecies=>BOOL,` | Write species as BNGL strings.<br>**Default**: `1` | 2.2.0 |
| `overwrite=>BOOL`<br>`})` | Overwrite existing files.<br>**Default**: `1` | 2.2.0 |
| `writeMDL({` | Write reaction network in MDL format for CellBlender/MCell. | 2.2.5 |
| `prefix=>"STRING",` | Set prefix of output file name.<br>**Default**: *model name* | 2.2.5 |
| `suffix=>"STRING"`<br>`})` | Set suffix of output file name.<br>**Default**: *N/A* | 2.2.5 |
| `writeModel({})` | Write model in BNGL format.<br>*Inherits all arguments from* `writeFile`, *with the following defaults*:<br>`format=>"bngl",`<br>`include_model=>1,`<br>`include_network=>0,`<br>`evaluate_expressions=>0,`<br>`pretty_formatting=>1,`<br>`overwrite=>0` | 2.2.0 |
| `writeNetwork({})` | Write reaction network in NET format.<br>*Inherits all arguments from* `writeFile`, *with the following defaults*:<br>`format=>"net",`<br>`include_model=>0,`<br>`include_network=>1,`<br>`evaluate_expressions=>0,`<br>`pretty_formatting=>0,`<br>`overwrite=>0` | 2.2.0 |

| | | |
|---|---|---|
| `visualize({` | Produce a model visualization in graph modeling language (GML) format. | 2.2.6 |
| `type=>"STRING",` | Set visualization type as `"contactmap"`, `"regulatory"`, `"ruleviz_operation"`, or `"ruleviz_pattern"`.<br>**Default**: `"regulatory"` | 2.2.6 |
| `help=>BOOL,` | Display the help menu.<br>(`visualize({type=>"TYPE",help=>1})` *displays a* `TYPE`-*specific help menu.*)<br>**Default**: `0` | 2.2.6 |
| `suffix=>STRING,` | Set suffix of output file name.<br>**Default**: *N/A* | 2.2.6 |
| `each=>BOOL,` | Output rule visualizations to separate files (incompatible with `textonly=>1`).<br>(`"ruleviz_pattern"`, `"ruleviz_operation"`, *and* `"regulatory"` *only.*)<br>**Default**: `0` | 2.2.6 |
| `background=>BOOL,` | Include background nodes in the graph.<br>(`"regulatory"` *only.*)<br>**Default**: `0` | 2.2.6 |
| `collapse=>BOOL,` | Collapse grouped nodes to single nodes.<br>(`"regulatory"` *only*; requires `groups=>1`.)<br>**Default**: `0` | 2.2.6 |
| `filter=>BOOL,` | Filter the set of nodes using the provided options file.<br>(`"regulatory"` *only.*)<br>**Default**: `0` | 2.2.6 |
| `groups=>BOOL,` | Enable automated grouping of nodes.<br>(`"regulatory"` *only*; results depend on `background=>BOOL`.)<br>**Default**: `0` | 2.2.6 |
| `level=>INT,` | Number of levels deep the graph should be explored during filtering.<br>(`"regulatory"` *only.*)<br>**Default**: `1` | 2.2.6 |
| `opts=>["STRING",...],` | List of text files with options for background, filtering, and groups.<br>(`"regulatory"` *only.*)<br>**Default**: *N/A* | 2.2.6 |
| `textonly=>BOOL` | Output a human-readable text file.<br>(`"regulatory"` *only.*)<br>**Default**: `0` | 2.2.6 |
| `})` | | |

Table S3: New actions and arguments (comma-separated format) introduced in the BioNetGen 2.2.x series of releases. STRING is any string of characters (must be enclosed in quotes); FLOAT is any real-valued number; <...> denotes an optional argument. Actions introduced prior to version 2.2.0 are labeled "< 2.2.0". For a complete list of all BioNetGen actions and arguments, see http://bionetgen.org/index.php/BNG_Actions_Args.

| action(arg1,arg2,...) | Description | Introduced |
|---|---|---|
| setModelName("STRING") | Set the model name.<br>*Default is the BNGL file basename.* | 2.2.0 |
| addConcentration("STRING",FLOAT) | Add to the concentration of a species.<br>*Value of* FLOAT *can be positive or negative.* | 2.2.0 |
| saveConcentrations(<"STRING">) | Store the current species concentrations.<br>*Optional* "STRING" *label can be specified for later reference.* | < 2.2.0<br>(*Labels in* 2.2.0) |
| resetConcentrations(<"STRING">) | Restore species concentrations.<br>*Unless an optional* "STRING" *label is provided, concentrations are restored to those from the last* saveConcentrations *command, or to the initial concentrations if* saveConcentrations *has not yet been called.* | < 2.2.0<br>(*Labels in* 2.2.0) |
| saveParameters(<"STRING">) | Store the current parameter values.<br>*Optional* "STRING" *label can be specified for later reference.*<br>*NOTE: Only constant parameters are saved, not derived parameters (expressions of constant parameters); see* resetParameters. | 2.2.0 |
| resetParameters(<"STRING">) | Restore parameter values.<br>*Unless an optional* "STRING" *label is provided, values are restored to those from the last* saveParameters *command, or to the initial values if* saveParameters *has not yet been called.*<br>*NOTE: Only constant parameters are restored, derived parameters are recalculated; see* saveParameters. | 2.2.0 |

# BioNetGen Quick Reference Guide



## Description

BioNetGen (bionetgen.org) is software for the specification and simulation of rule-based models of biochemical systems, including signal transduction, metabolic, and genetic regulatory networks. The rule-based approach allows for the maintenance of detailed information on molecular structures and interactions, as well as significant scalability both in model construction and simulation.

## Installation

1. Download RuleBender, a Graphical User Interface for BioNetGen (rulebender.org).
2. Java: If needed, install Java version 1.6 or greater from the Oracle download site (oracle.com/java).
3. Perl: Perl is installed on most Unix-like operating systems. You may need to install it on Windows. We recommend ActivePerl.

## Required Model Components

| *Block Name* | *Description* |
|---|---|
| `parameters` | Values and expressions for parameters in the model. |
| `molecule types` | Molecule definitions including components and component states. |
| `seed species` | Initial conditions for molecules and complexes present at simulation start time. |
| `observables` | Sums over concentrations of species with properties specified using patterns. |
| `functions` | Functions of observables used to construct non-elementary rate laws that depend on global or local properties. |
| `reaction rules` | Generate reactions with the specified rate law based on selecting and transforming reactants using patterns. |
| `actions` | Sequence of actions used to simulate the model. |

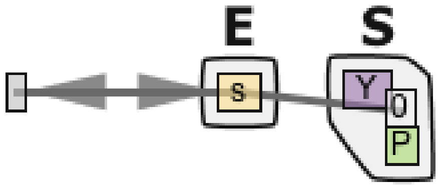


## Contact Map

Shows the molecules, components, component states and bonds, as well as synthesis and deletion of molecules. Right-clicking on molecules allows the user to search for similarly named proteins in a number of established databases.

## Example BNGL Model

```
# MM Example
begin model
begin parameters
    # Avogadro's number - scaled for umol
    NA   6.022e23/1e6
    # Cell volume
    V    1e-12 # liters - typical for eukaryote
    # Rate constants
    kp1  1.0/(NA*V) # 1/uM 1/s -> 1/molecules 1/s
    km1  0.1 # 1/s
    k2   0.01 # 1/s
    ksyn 1e-4*(NA*V) # uM/s -> molecules / s
    kdeg 0.01 # 1/s
    # Initial concentrations
    E0   0.01*NA*V # uM -> molecules
    S0   1.0*NA*V  # uM -> molecules
end parameters
begin molecule types
    E(s)
    S(Y~0~P)
end molecule types
begin seed species
    E(s)   E0
    S(Y~0) S0
end seed species
begin observables
    Molecules SU S(Y~0)
    Molecules SP S(Y~P)
    Molecules ES E(s!1).S(Y!1)
    Molecules Etot E()
end observables
begin reaction rules
    ESbind: E(s) + S(Y~0) <-> E(s!1).S(Y~0!1) kp1,km1
    ESconvert: E(s!1).S(Y~0!1) -> E(s) + S(Y~P) k2
    Esyndeg: 0 <-> E(s) ksyn, kdeg
end reaction rules
end model
# actions
generate_network({overwrite=>1})
visualize({type=>"regulatory",groups=>1,\
           collapse=>1,opts=>"opts.txt"})
simulate({method=>"ode",t_end=>20000,n_steps=>1000})
```

## Simulation Results

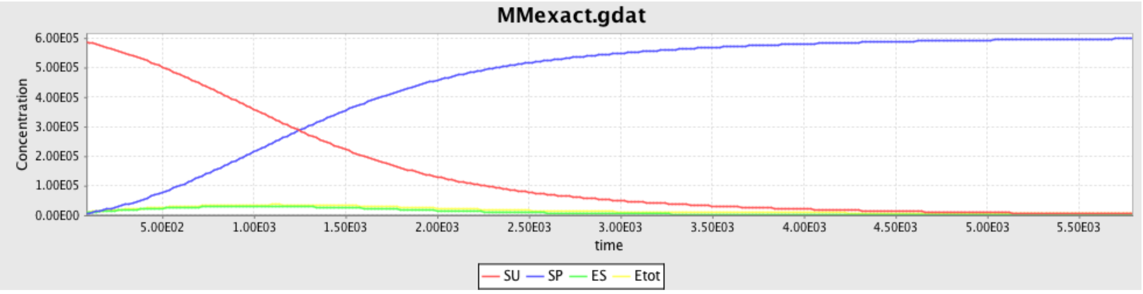

**Compartmental BioNetGen** (bionetgen.org/index.php/Compartments_in_BNGL)
Extension of BNGL to enable explicit modeling of the compartmental organization of the cell and its effects on system dynamics. Introduces localization attributes for both molecules and species, as well as appropriate volumetric scaling of reaction rates.

```
begin compartments
    EC  3  vol_EC              # extracellular space
    PM  2  sa_PM*eff_width  EC  # plasma membrane
    CP  3  vol_CP           PM  # cytoplasm
    NM  2  sa_NM*eff_width  CP  # nuclear membrane
    NU  3  vol_NU           NM  # nuclear space
    EM  2  sa_EM*eff_width  CP  # endosomal membrane
    EN  3  vol_EN           EM  # endosomal space
end compartments
```

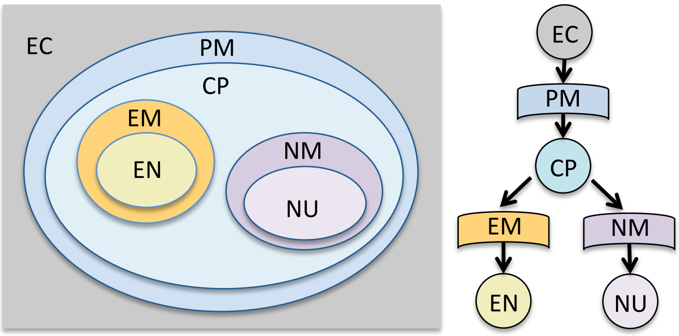


**Context and Pattern Matching within Rules**
Context (shown below in red) encompasses components, states, and bonds in a rule that do not undergo transformation.

| *Reaction Rule* | *Reactant Requirements* | *Reactant Species Matched* |
|---|---|---|
| `R1: R(l!+,Y~0) -> R(l!+,Y~P)  k1` | R must be unphosphorylated at Y and bound at l (binding site for L). | `R(l!1,Y~0).L(r!1)` |
| `R2: R(l,Y~0) -> R(l,Y~P)  k2` | R must be unphosphorylated at Y and *not* bound at l. | `R(l,Y~0)` |
| `R3: R(Y~0) -> R(Y~P)  k3` | R must be unphosphorylated at Y. | `R(l!1,Y~0).L(r!1)`<br>`R(l,Y~0)` |

Context restricts the application of a given rule. Rules with more context are more specific and rules with less context are more general. Using more context allows for greater control over rates of specific reactions at the cost of requiring more rules to specify a model. Here, R1 and R2 specify different phosphorylation rates depending on whether R is bound at l, whereas R3 specifies a rate that is independent of the state of l.

**Functional Rate Laws** (bionetgen.org/index.php/Functions)
A function is a mathematical expression that can involve numbers, parameters, observables, and other pre-defined functions and operators (see bionetgen.org/index.php/Built-ins). Functions can be used to define reaction rules that do not obey mass-action kinetics. Importantly, functions *substitute* for rate constants, meaning that the rate of a reaction is calculated as the product of the function and the reactant species concentrations (analogous to mass-action rate laws). Functions can be defined "inline" following a reaction rule or within a separate block of the BNGL file, with the following syntax (`[...]` denotes an optional argument):

```
  begin functions
     [label:]  func_name([arg]) [=] math_expression
         ⋮
  end functions
```

Here, `arg` is a "pointer" to a specific complex or molecule and limits the scope over which observables within the function definition are calculated (the default scope is the entire system). Functions that do not accept an argument are termed "global functions" and those that do are termed "local functions." Pointers to complexes and molecules are specified by "tagging" a reactant pattern in a rule using the `%tag` syntax, where `tag` can be any alphanumeric string of characters. Tags prefixed to a pattern (e.g., `%x:A()`) point to the *complex* matched by the pattern and tags postfixed (e.g., `A()%x`) point to the matched *molecule*.

*Examples*:

```
begin observables
   Molecules  Atot  A()                     # Observable counting total number of A molecules
   Molecules  Bp    B(c~P)                  # Observable counting number of phosphorylated B molecules
end observables
begin functions
   gfunc() = 0.5*Atot^2/(10+Atot^2)         # Hill function (global) defined over all A molecules in the system
   lfunc(x) = 0.5*Atot(x)^2/(10+Atot(x)^2)  # Hill function (local) defined over all A molecules in "x"
end functions
begin reaction rules
   B(c) + C(b) -> B(c!1).C(b!1) gfunc()            # Binding rate depends on no. of A molecules in the system
   B(c) + C(b) -> B(c!1).C(b!1) 0.5*Atot^2/(10+Atot^2)  # Ditto, but with "inline" function definition
   %y:B(c) + C(b) -> %y:B(c!1).C(b!1) lfunc(y)     # Prefix tag limits observable scope to complex containing B
   B(c)%y + C(b) -> B(c!1)%y.C(b!1) Bp(y)*gfunc()  # Postfix tag limits observable scope to B molecule only
end reaction rules
```

## Maintaining Consistent Units

Units are not enforced within BioNetGen, but for realistic results units among all concentrations and rate constants must be kept consistent. The most common units utilized are in terms of molecules/cell. ($N_A$: Avogadro's number; $V$: volume)

| *Common Parameters* | *Example Starting Value* | *Desired Units* | *Conversion Factor* | *Final Parameter* |
|---|---|---|---|---|
| Volumes | $10^{-6}$ $\mu$l | l | $10^{-6}$ l/$\mu$l | $10^{-12}$ l |
| Concentrations | 0.01 $\mu$M | molec | $N_A \times V/10^6$ molec/$\mu$M | 6022 molec |
| 1st-order rate constants | 1 $s^{-1}$ | $s^{-1}$ | *None* | 1 $s^{-1}$ |
| 2nd-order rate constants | $10^5$ $M^{-1}s^{-1}$ | $molec^{-1}s^{-1}$ | $1/(N_A \times V)$ M/molec | $1.66 \times 10^{-7}$ $molec^{-1}s^{-1}$ |

## Reading Models from File

In addition to `.bngl` files, BioNetGen can read in pre-generated reaction networks from `.net` files and SBML models with the `.xml` extension. This is done using the `readFile({file=>"filename"})` action. Optional arguments include `blocks=>["blockname1", "blockname2",...]` and `atomize=>0/1`. If the filename ends with `.xml`, the SBML-to-BNGL translator is automatically called. The `atomize=>1` option invokes the "Atomizer," a method for extracting implicit molecular structure from flat SBML species. The Atomizer can also be accessed as a standalone web application at ratomizer.appspot.com/translate.

## Simulation Methods

| *Method* | *Command* | *Description* |
|---|---|---|
| Ordinary differential equations | `simulate({method=>"ode"})` | Network-based deterministic simulation using the SUNDIALS CVODE ODE solver. |
| Stochastic simulation algorithm | `simulate({method=>"ssa"})` | Network-based stochastic simulation using the Gillespie direct method to sample over reactions. |
| Partitioned-leaping algorithm | `simulate({method=>"pla"})` | Network-based stochastic simulation using a tau-leaping variant to speed up simulation. |
| Network-free simulation | `simulate({method=>"nf"})` | Stochastic simulation that does not require network generation. Uses the Gillespie direct method to sample over reaction rules. Scalable to models encoding large reaction networks (see nfsim.org for more information). |

## Parameter Scans

BioNetGen allows the user to run parameter scans, which quantify the effects of varying the value of an individual parameter on any observable species. This is done using the command `parameter_scan({argument=>value})` with the following arguments:

| *Argument* | *Usage* | *Example* |
|---|---|---|
| `parameter` | Name of the parameter to be varied. | `parameter=>"kp1"` |
| `par_min` | Minimum value the parameter will take. | `par_min=>1e-3` |
| `par_max` | Maximum value the parameter will take. | `par_max=>1e3` |
| `n_scan_pts` | Number of values the parameter will take, uniform between `par_min` and `par_max`. | `n_scan_pts=>1000` |
| `log_scale` | Selects parameter values uniformly between $\log_{10}$(`par_min`) and $\log_{10}$(`par_max`). | `log_scale=>1` |
| `method` | Simulation method to be used (`"ode"`, `"ssa"`, `"pla"`, or `"nf"`). | `method=>"ode"` |
| `t_end` | Simulation run time. | `t_end=>10000` |
| `n_steps` | Number of observable outputs. | `n_steps=>1000` |

## Exporting Models to Other Formats

| *Action* | *File Extension(s)* | *Description* |
|---|---|---|
| `writeModel` | .bngl | BNGL model file. |
| `writeNetwork` | .net | Reaction network file used for network-based simulations. |
| `writeSBML` | .xml | Systems Biology Markup Language; compatible with many software packages. |
| `writeMfile` | .m | Model file compatible with Matlab. |
| `writeMexfile` | .cvode.c, .m | Model file written in C that can be compiled into a Matlab executable (MEX) file. |
| `writeXML` | .xml | Model file usable for network-free simulation in NFsim. |
| `writeMDL` | .mdl, .py, .geometry.mdl | Model file usable for spatial simulations in MCell. |
| `visualize` | .gml | Graph Modeling Language file for visualizations. |

**Energy Modeling in BioNetGen** (http://bionetgen.org/index.php/Energy_Modeling)
Extension of BNGL to enable definition of energy patterns to drive model kinetics based on changes in free energy of reactions. Typically allows for the writing of fewer rules for each model, less context in each rule, and the generation of reaction networks guaranteed to satisfy detailed balance.

**Visualization** (bionetgen.org/index.php/Visualization)
Visualization tools are accessed using one or more `visualize({type=>"string"})` commands. Optional arguments include `each=>1` to generate a separate output file for each rule and `suffix=>"string"` to append a suffix to the file name. The output is a Graph Modeling Language file `[model]_[type]_[suffix].gml`, which can be processed by graph layout software such as yEd (yworks.com/yed).

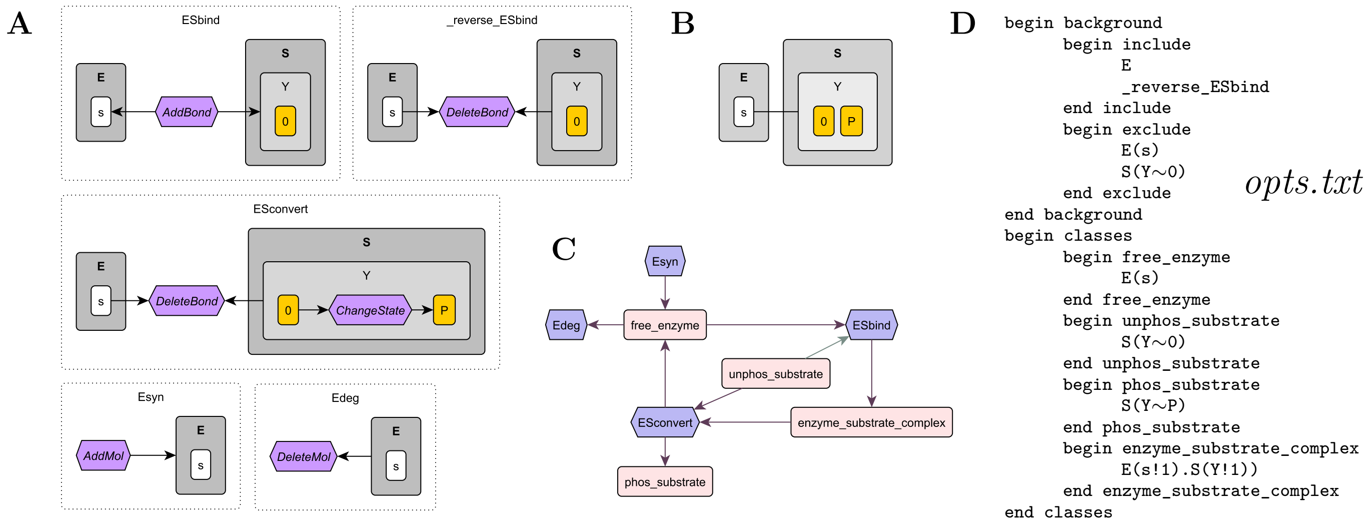


**A. Rule visualization:** Rules can be visualized either in terms of graph operations (`type=>"ruleviz_operation"`) or reactant and product patterns (`type=>"ruleviz_pattern"`).
*Command used here*: `visualize({type=>"ruleviz_operation"})`.

**B. Contact map:** Equivalent to the contact maps generated by RuleBender (except for the synthesis/degradation directed edges).
*Command used here*: `visualize({type=>"contactmap"})`.

**C. Regulatory graph:** Graphical representation of the basic processes in a model. Here, processes are grouped (`groups=>1`) and group nodes are collapsed (`collapse=>1`) into single nodes. Additional options exist for displaying hidden sites and processes (`background=>1`) and for outputting the visualization to a human-readable text file (`textonly=>1`).
*Command used here*: `visualize({type=>"regulatory",groups=>1,collapse=>1,opts=>"opts.txt"})`.

**D. User options:** For regulatory graphs, user-defined commands can be specified in text files and loaded using `opts=>"filename"` or `opts=>["filename1","filename2",...]`. Useful for modifying the background and providing intuitive names to groups of sites.
